# Supplementary material for: Seeing with Humans: Gaze-Assisted Neural Image Captioning
Source: arXiv:1608.05203 ancillary file (2016-08-18)
Supplement: Supplementary file 1 [file supplementary.pdf]

# Seeing with Humans: Gaze-Assisted Neural Image Captioning
## – Supplementary Material –

Yusuke Sugano and Andreas Bulling

## Comparison of attention allocation results

Each line shows the input image and the attention map examples at each step together with their corresponding output words.

### Object Discovery

Gaze information typically helps the model to find small important objects from cluttered scenes. This also happens when the important object is not located in the center of the image. In the following, the output from the baseline model is shown first, and the gaze-assisted model follows.

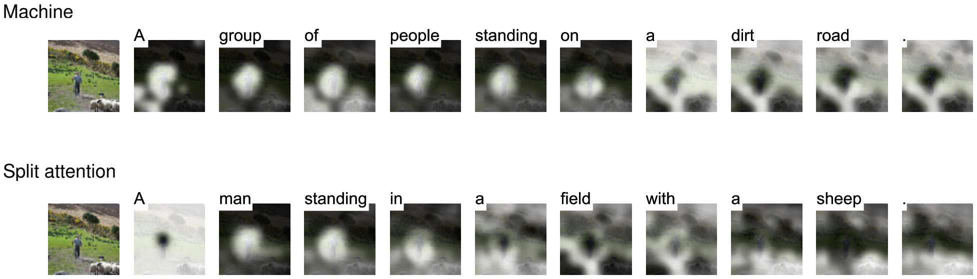


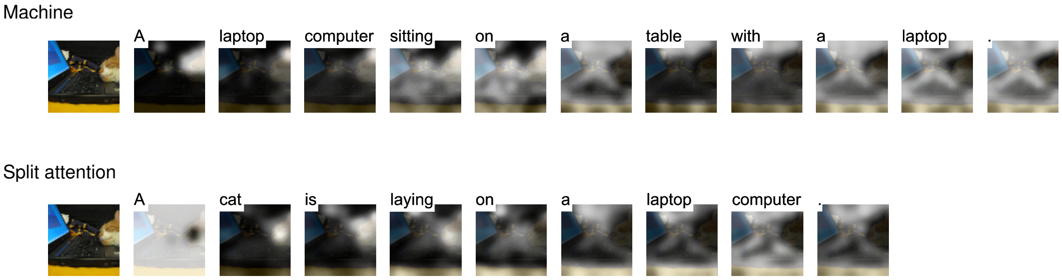


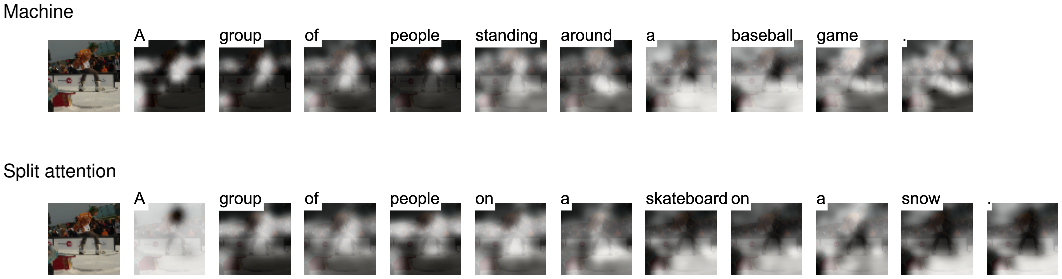


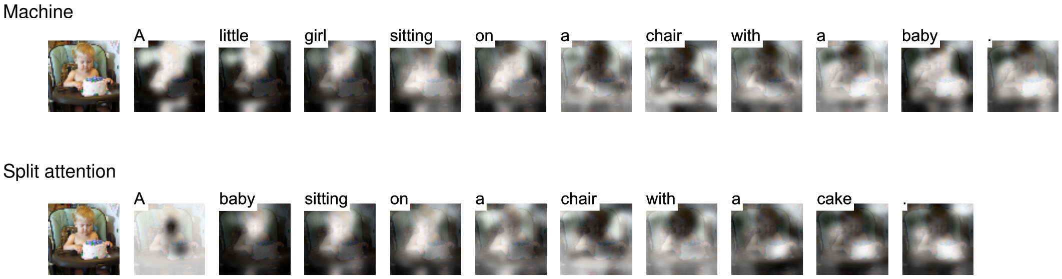

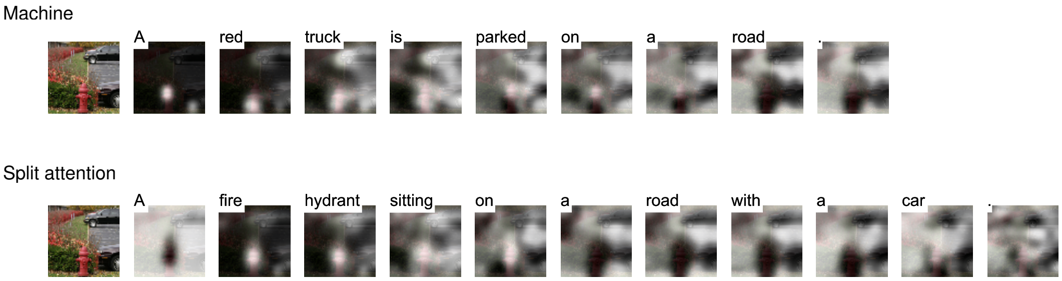


## Repetitive Descriptions

The baseline model often generates repetitive descriptions by separating a single object entity into multiple image regions. In contrast, gaze-assisted model discovers clearer object regions of interest, and avoids attending to the same object more than twice.

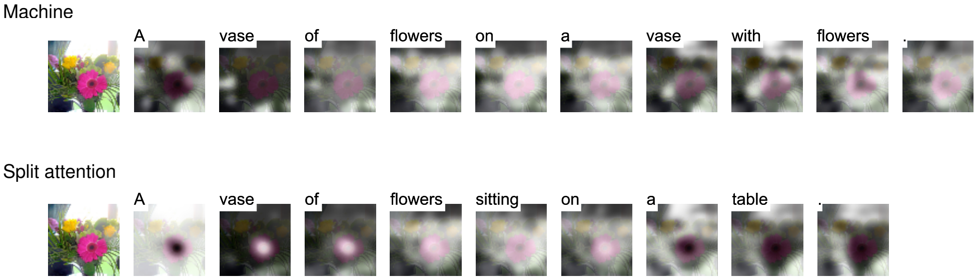


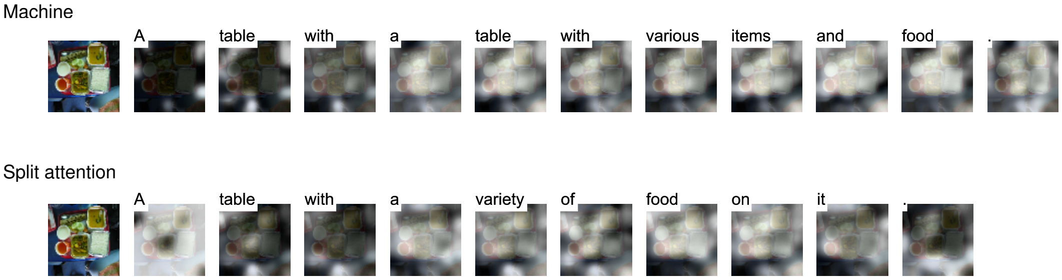


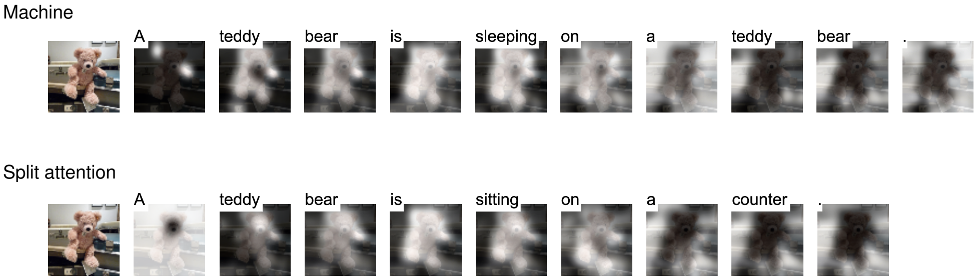


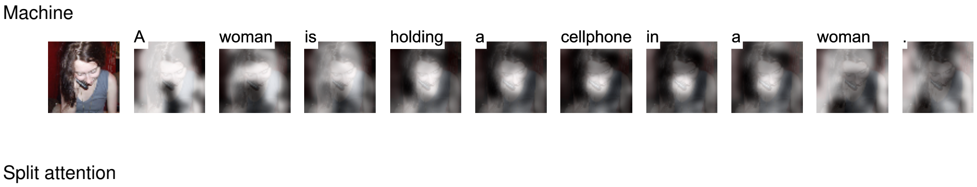

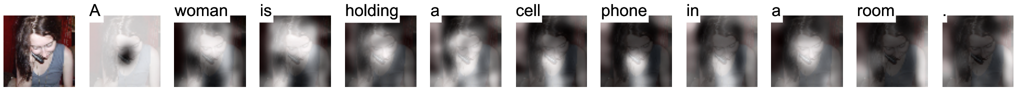


Machine

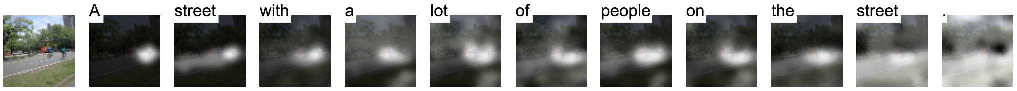


Split attention

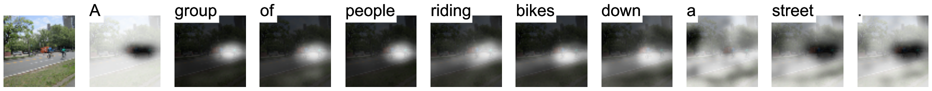


### Effect of Split Attention

While gaze feature alone can help the model to find important objects, there are some objects which do not attract human fixations. Humans also do not fixate on background regions. Our proposed split attention model allows the model to flexibly allocate attention to non-fixated regions too, and improves failure cases of the gaze-only model purely relying on gaze feature missing non-fixated objects and background scene categories. In the following, the output from the baseline model, the gaze-only model without non-fixated attention term, and the proposed split attention model is shown.

Machine

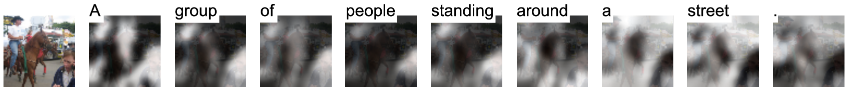


Gaze-only

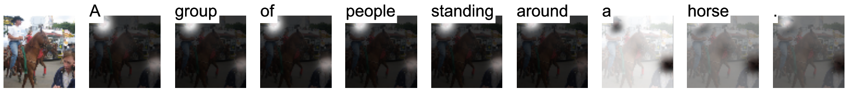


Split attention

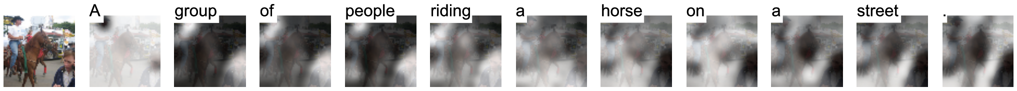


Machine

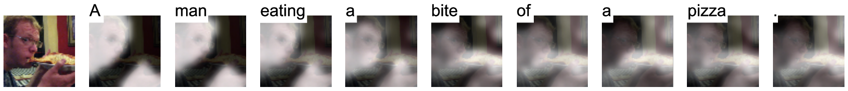


Gaze-only

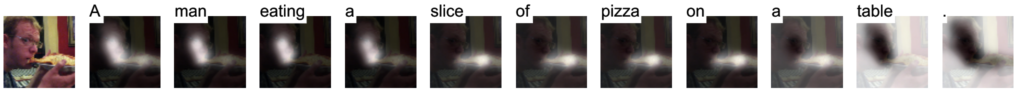


Split attention

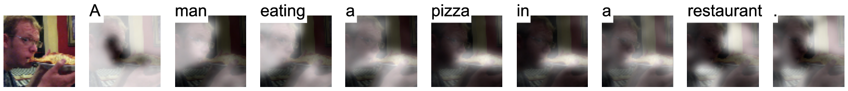


Machine

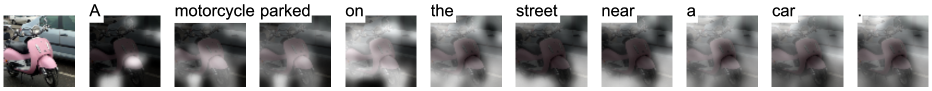

Gaze-only

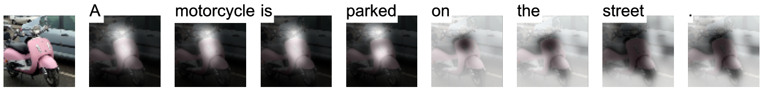


Split attention

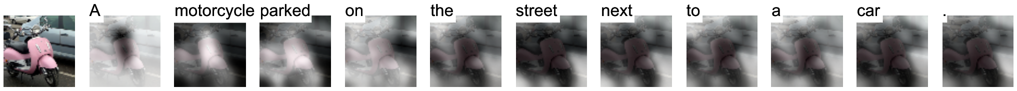


Machine

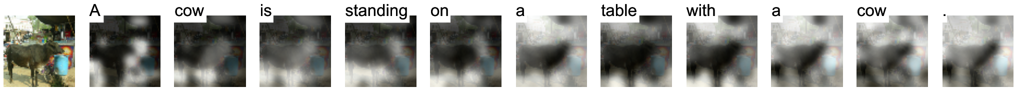


Gaze-only

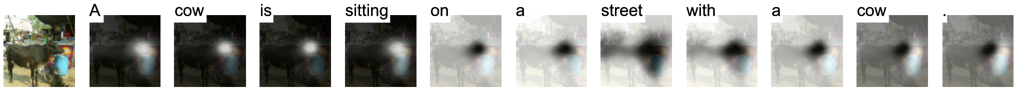


Split attention

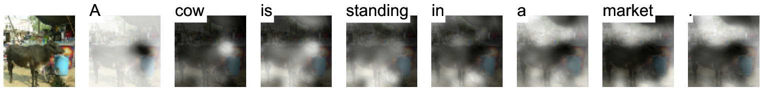


Machine

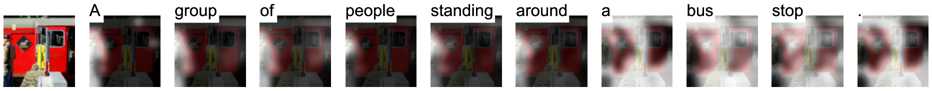


Gaze-only

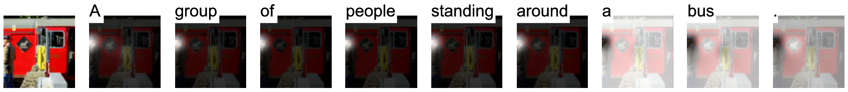


Split attention

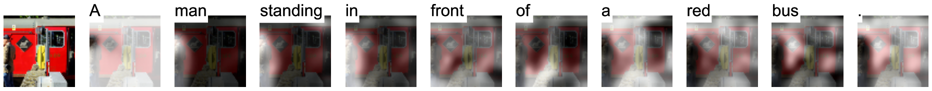


Machine

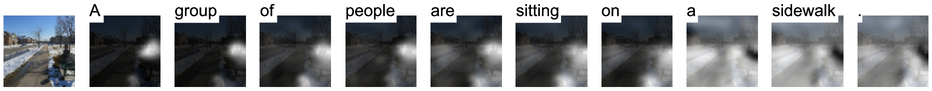


Gaze-only

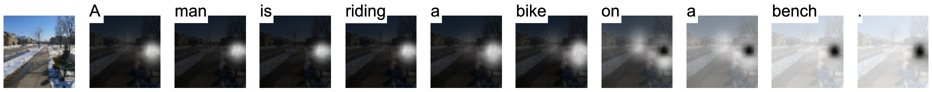


Split attention

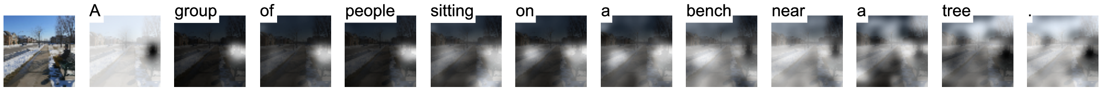


Machine

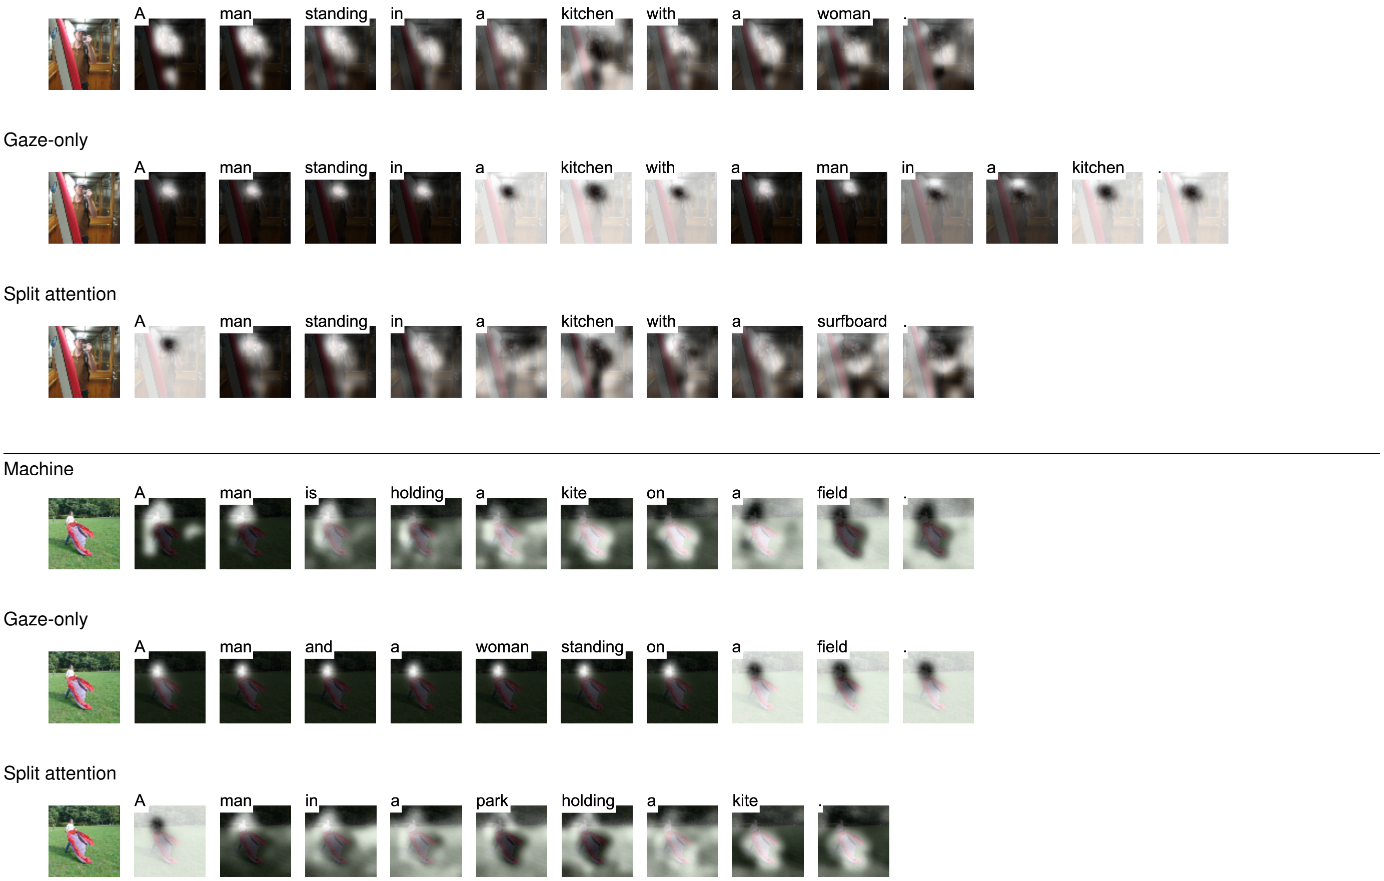
A man standing in a kitchen with a woman .
Gaze-only
A man standing in a kitchen with a man in a kitchen .
Split attention
A man standing in a kitchen with a surfboard .
Machine
A man is holding a kite on a field .
Gaze-only
A man and a woman standing on a field .
Split attention
A man in a park holding a kite .
